# Supplementary material for: MACQ: A Holistic View of Model Acquisition Techniques
Source: arXiv:2206.06530 source file (2022-06-14)
Supplement: Supplementary file 1 [file appendix.tex]

% \newpage
% \onecolumn
% \appendix
% \section{Example \macq Usage}

% \vspace{1em}
% Here, we show one example usage of the \macq library.
%
